# Supplementary material for: Electric quadrupole and magnetic dipole coupling in plasmonic nanoparticle arrays
Source: arXiv:1802.07960 ancillary file (2018-02-22)
Supplement: Supplementary file 1 [file Supporting_Information.pdf]

# Supporting Information for

## Electric quadrupole and magnetic dipole coupling in plasmonic nanoparticle arrays


Viktoriia E. Babicheva[1,]* and Andrey B. Evlyukhin[2]

[1]*College of Optical Sciences, University of Arizona, Tucson, AZ, USA*

[2]*Laser Zentrum Hannover e.V., Hollerithallee 8, D-30419, Hannover, Germany*

*ITMO University, 49 Kronverksky Ave., St. Petersburg, 197101, Russia*

**email:* vbab.dtu@gmail.com


### Supporting-Information Figure S1

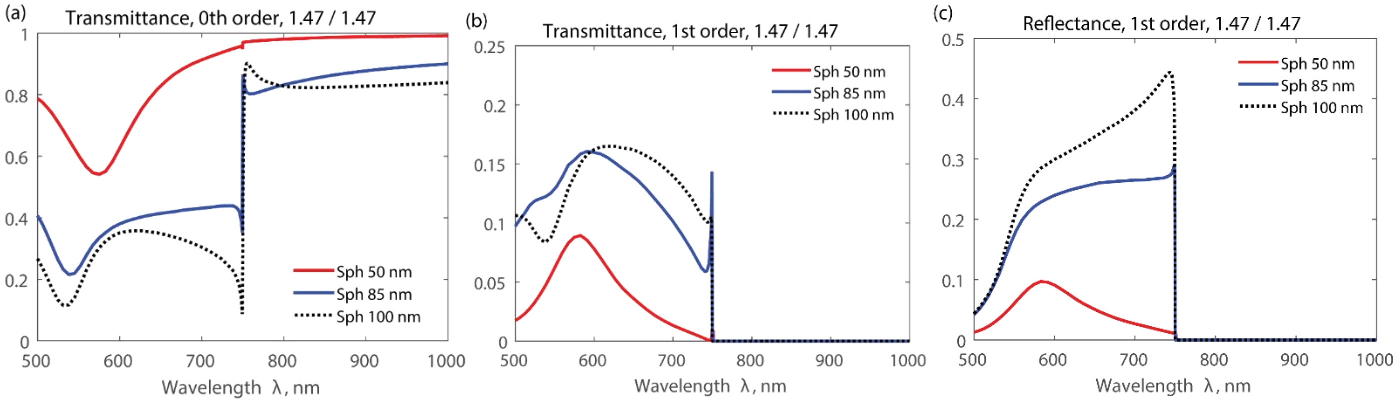


Fig. S1. Transmittance in the zeroth (a) and the first (b) diffraction orders and reflectance in the first (c) diffraction orders of the nanosphere array. Periods are $p_x$ = 510 nm and $p_y$ = 250 nm, the environment is homogeneous with $n = n_s$ = 1.47, and numbers denote radius $R$ of the sphere.

### Supporting-Information Figure S2

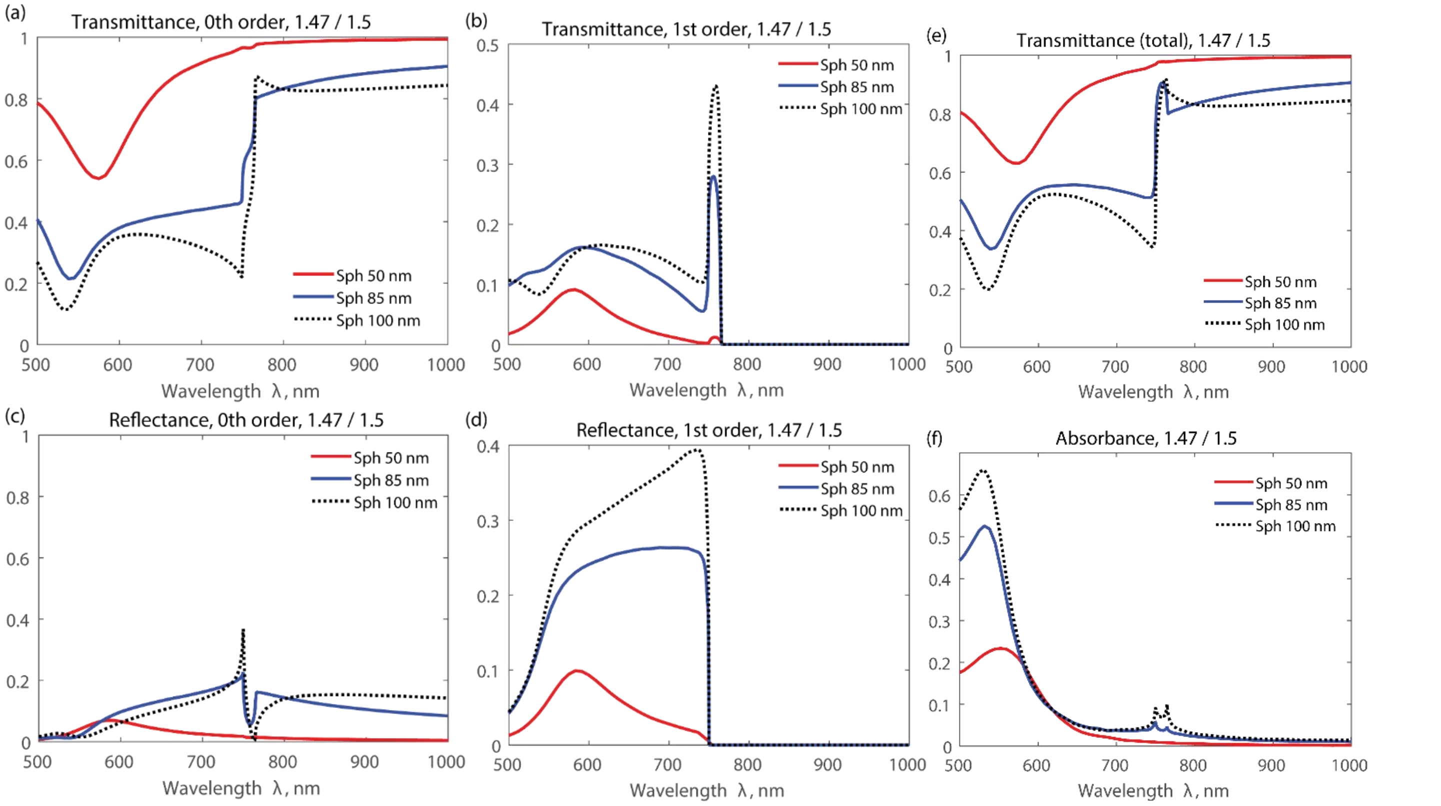


Fig. S2. Nanosphere array in the non-homogeneous environment: transmittance in the zeroth (a) and the first (b) diffraction orders and reflectance in the zeroth (c) and the first (d) diffraction orders; (e) total transmittance; (f) Absorbance. Periods are $p_x$ = 510 nm and $p_y$ = 250 nm. The refractive indices of the superstrate and the substrate are $n_s$ = 1.47 and $n$ = 1.5, respectively. Numbers denote the sphere radius.

## Supporting-Information Figure S3

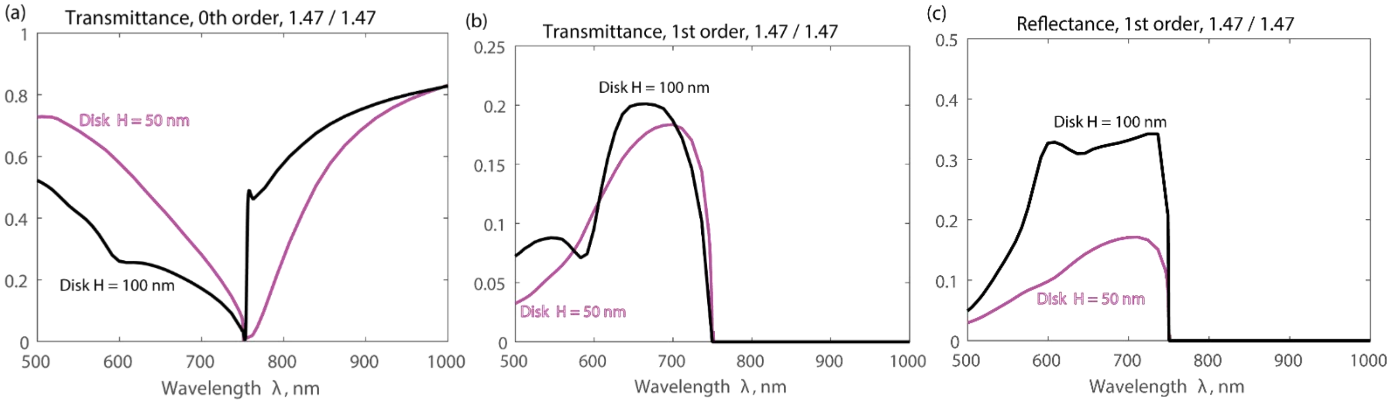


Fig. S3. Transmittance in the zeroth (a) and the first (b) diffraction orders and reflectance in the first (c) diffraction orders of the nanodisk array. Periods are $p_x$ = 510 nm and $p_y$ = 250 nm, the environment is homogeneous with $n = n_s = 1.47$, height $H$ of the disk is either 50 or 100 nm, and its radius $R_d$ = 85 nm.

## Supporting-Information Figure S4

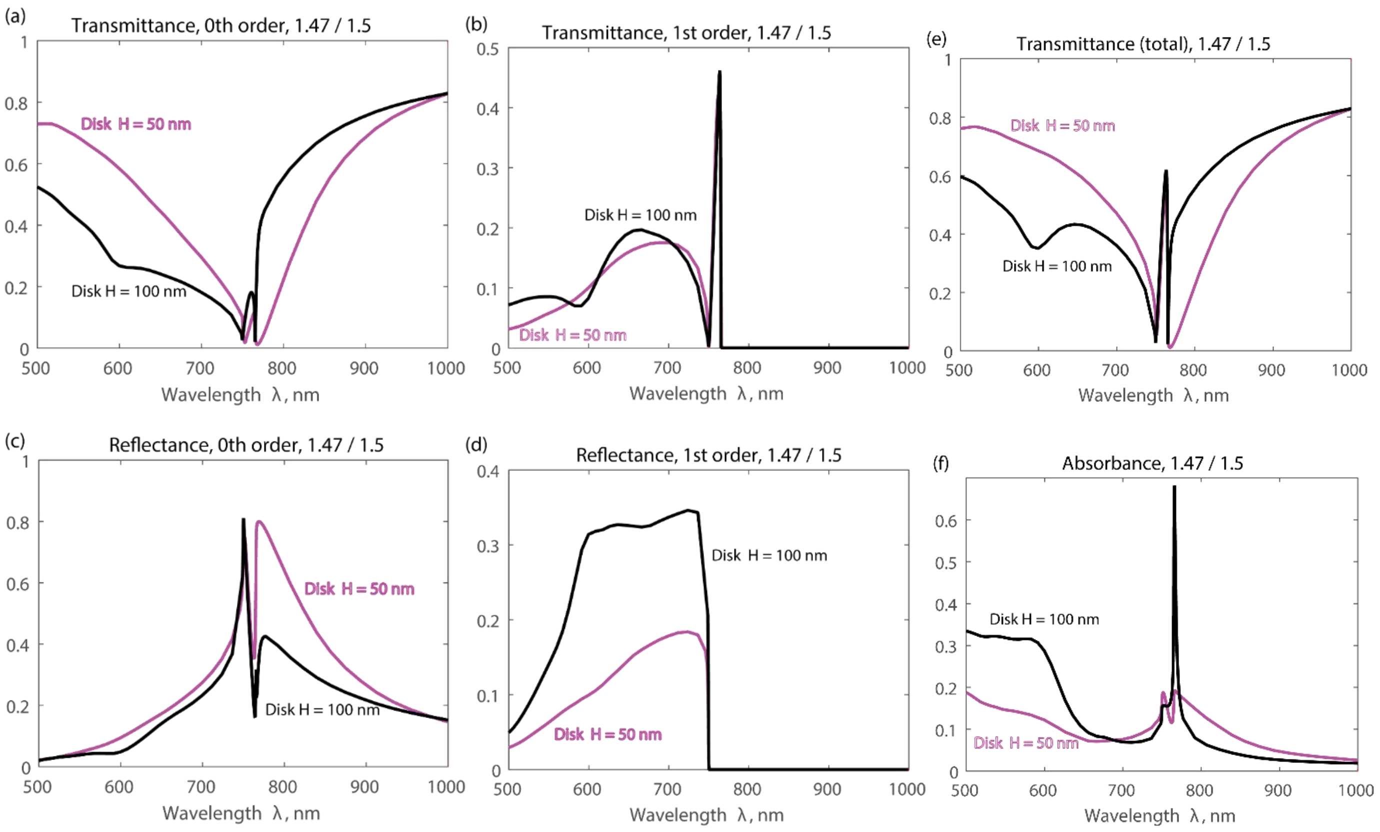


Fig. S4. Nanodisk array in the non-homogeneous environment: transmittance in the zeroth (a) and the first (b) diffraction orders and reflectance in the zeroth (c) and the first (d) diffraction orders; (e) total transmittance; (f) Absorbance. Periods are $p_x$ = 510 nm and $p_y$ = 250 nm. The refractive indices of the superstrate and the substrate are $n_s$ = 1.47 and $n$ = 1.5, respectively. Height $H$ of the disk is either 50 or 100 nm, and its radius $R_d$ = 85 nm.

**Supporting-Information Figure S5**

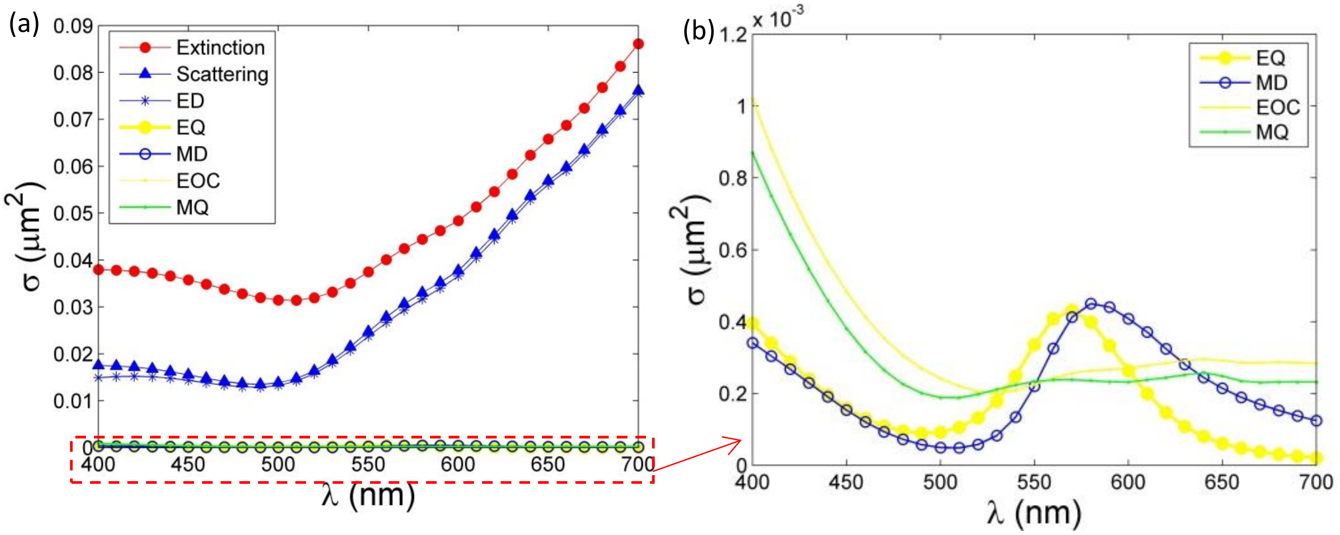


Fig. S5. (a) Total scattering cross-sections and multipole decomposition of the nanodisks with $R_d$ = 85 nm and $H$ = 50 nm in a homogeneous environment with $n = n_s = 1.47$ calculated using a discrete dipole-quadrupole approximation. (b) An enlarged view of EQ, MD, EOC, and MQ, which have much smaller value than ED.

**Nanoparticle array in the non-homogeneous environment:**

1) In the first diffraction order of transmission, the peak is broader and more pronounced;
2) In the zeroth diffraction order of transmission, the resonances are weaker and smeared out;
3) In the zeroth diffraction order of reflection, the feature is broader and stronger;
4) In the first diffraction order of reflection, there is no feature.

**Supporting-Information Figure S6**

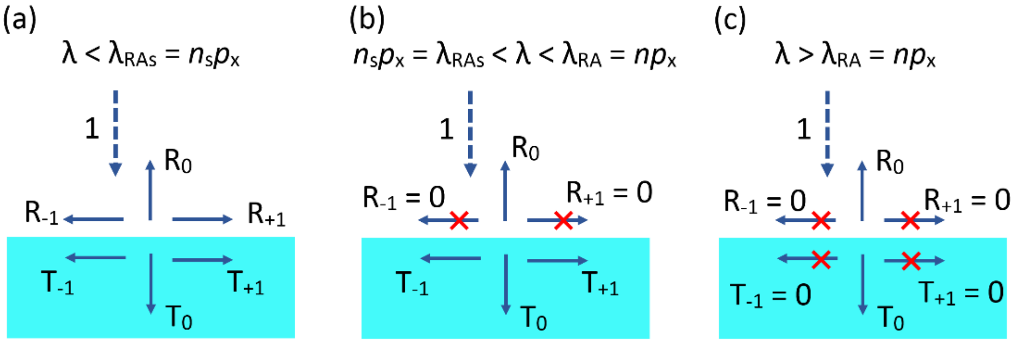


Fig. S6. Schematic view of transmission and reflection in the zeroth ($T_0$ and $R_0$) and the first diffraction orders ($T_{\pm1}$ and $R_{\pm1}$) for different wavelengths (shown in panels) in the case $n_s < n$. While Rayleigh anomaly is a complex process and results in non-monotonic spectra, for simplicity, we use notations $\lambda_{RA} = np_x$ and $\lambda_{RAs} = n_s p_x$. For the case $n_s < n$ and $\lambda < \lambda_{RAs}$, both reflection and transmission into the first diffraction order are allowed and non-zero. Next, for $\lambda_{RAs} < \lambda < \lambda_{RA}$, the first diffraction order of reflection is suppressed. Finally, for $\lambda > \lambda_{RA}$, both the first diffraction orders of reflection and transmission vanish. When the first order disappears in the superstrate, a lattice mode of the structure is excited and it couples to the substrate, which results in an increase of transmission and suppression of reflection.

**Supporting-Information Figure S7**

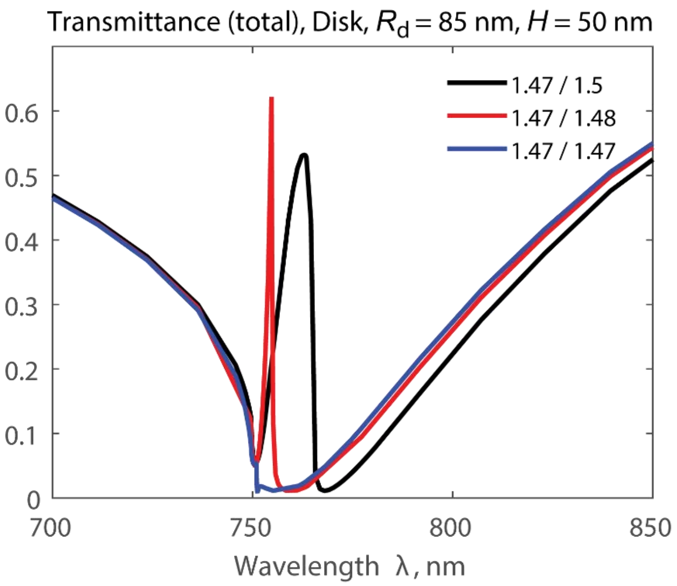


Fig. S7. The transmittance of the array of nanodisks with $R_d$ = 85 nm and $H$ = 50 nm with a small difference between the refractive indices of the substrate and the superstrate (denoted in the legend). Periods are $p_x$ = 510 nm and $p_y$ = 250 nm.

**Supporting-Information Figure S8**

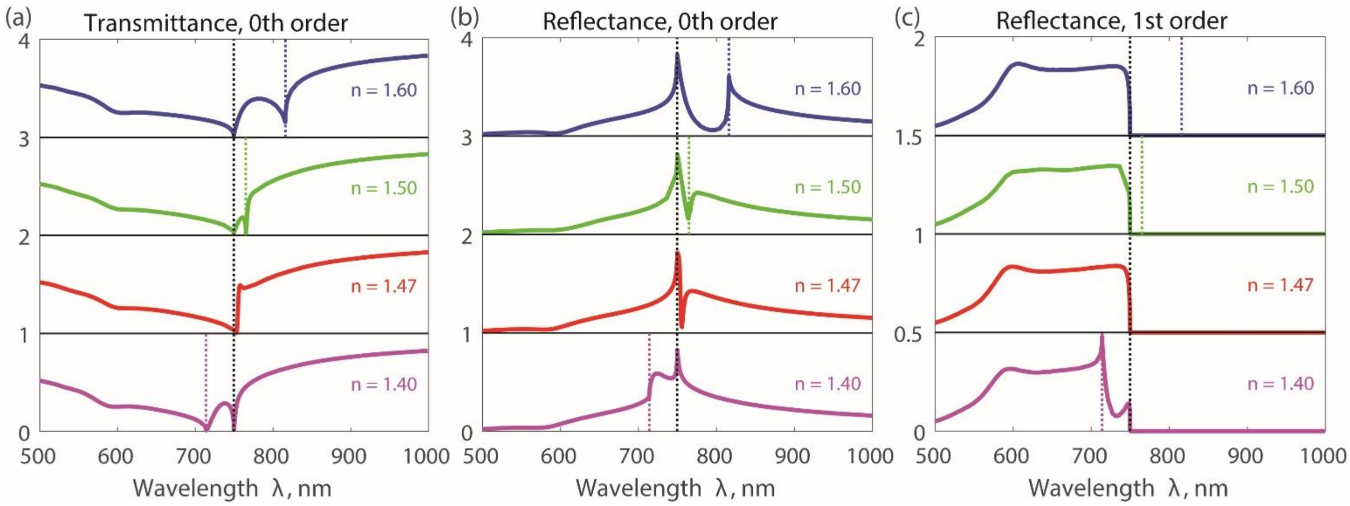


Fig. S8. (a) $0^{th}$ order transmittance, (b) $0^{th}$ order reflectance, and (c) $1^{st}$ order reflectance for nanodisks with $R_d$ = 85 nm and $H$ = 100 nm (see more results in Fig. 8). Periods are $p_x$ = 510 nm and $p_y$ = 250 nm, $n_s$ = 1.47. The dotted color lines mark a wavelength where the resonances in the substrate are expected, i.e. $\lambda_{RA} = np_x$, and the dotted black line corresponds to the resonance in superstrate, i.e. $\lambda_{RAs} = np_{xs}$. Each plot is shifted by either 0.5 or 1 with respect to the previous one.

The transmittance band between the anomalies for $n > n_s$ is associated with the transmission into the first diffraction order of the substrate (blue and green lines), and when this diffraction order disappears, the total transmission decreases. For $n < n_s$, the strong transmittance band does not exist between the Rayleigh anomalies. The spectra of the total reflection basically repeat the spectra of the zeroth diffraction order beam into the superstrate. Only in the case of $n < n_s$ the reflection into the first diffraction order can be significantly increased due to disappearing of the first diffraction order of the transmission (for $n$ = 1.40).

**Supporting-Information Figure S9**

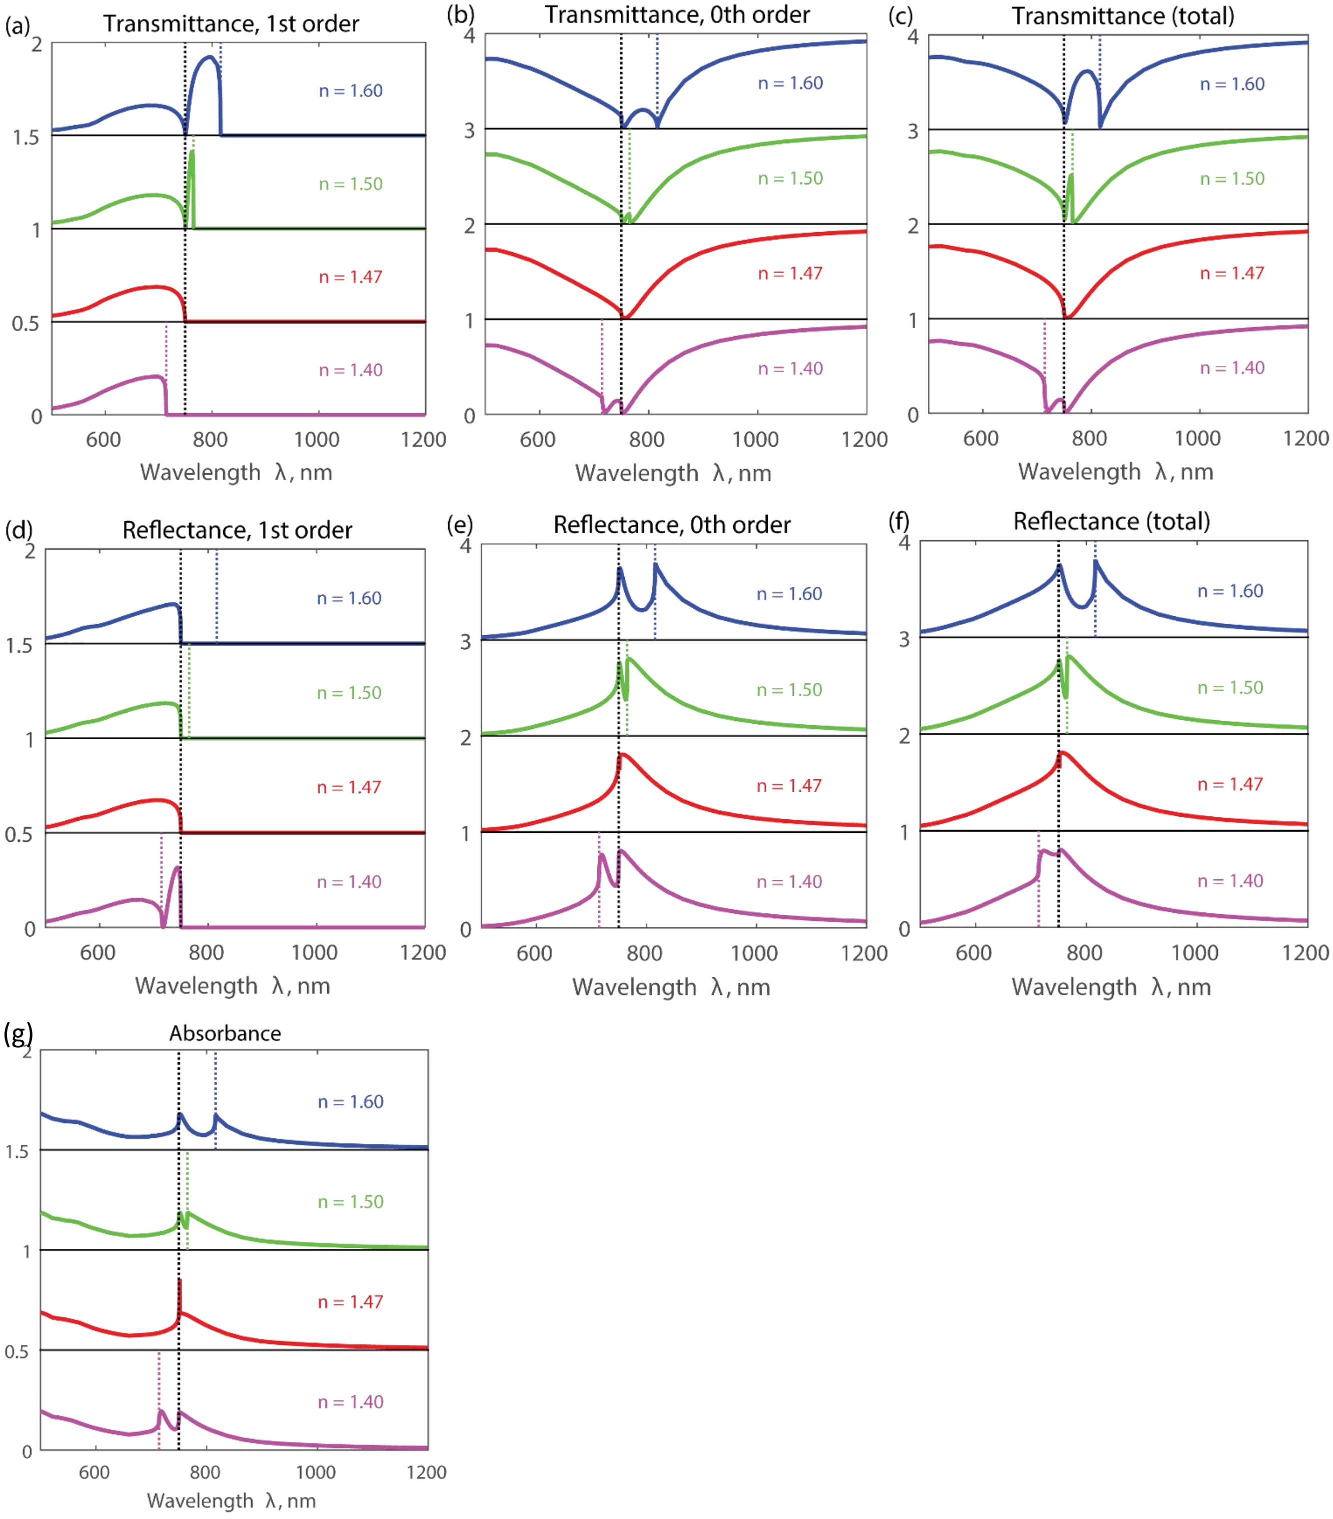


Fig. S9. (a)-(c) Transmittance, (d)-(f) reflectance, and (g) absorbance of the array of nanodisks ($R_d$ = 85 nm and $H$ = 50 nm) for different $n$ denoted on the plots. Periods are $p_x$ = 510 nm and $p_y$ = 250 nm, $n_s$ = 1.47. The dotted color lines mark a wavelength where the resonances in the substrate are expected, i.e. $\lambda_{RA} = np_x$, and the dotted black line corresponds to the resonance in superstrate, i.e. $\lambda_{RAs} = np_{xs}$. Each plot is shifted by either 0.5 or 1 with respect to the previous one.

Transmission in the first diffraction orders is either suppressed for $\lambda_{RAs} < \lambda < \lambda_{RA}$ and $n < n_s$ or has a peak for $\lambda_{RAs} < \lambda < \lambda_{RA}$ and $n > n_s$. As a result, both the zeroth diffraction order and the total transmittance for all $n \neq n_s$ under consideration have two minimums, i.e. at $\lambda_{RAs}$ and $\lambda_{RA}$. The first diffraction order of reflection has two features at $\lambda = \lambda_{RAs}$ and $\lambda = \lambda_{RA}$ and $n < n_s$ and it is suppressed at $\lambda_{RAs} < \lambda < \lambda_{RA}$ and $n > n_s$, which altogether causes two peaks in reflectance, the zeroth diffraction order and total, at $\lambda_{RAs}$ and $\lambda_{RA}$ for all $n$.

**Supporting-Information Figure S10**

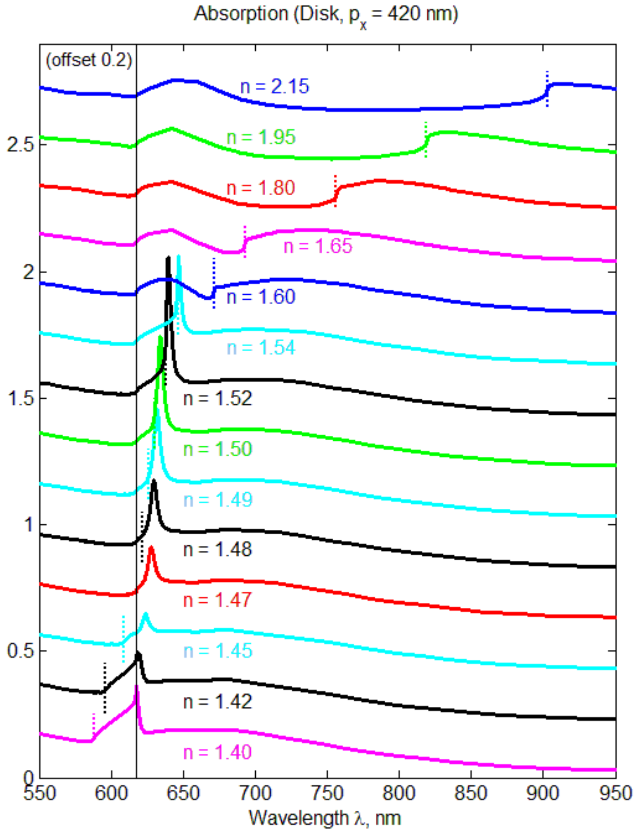


Fig. S10. Absorbance for various $n$. Periods are $p_x$ = 420 nm and $p_y$ = 250 nm, a disk with $R_d$ = 85 nm and $H$ = 50 nm, and $n_s$ = 1.47. The dotted color lines mark a wavelength where the resonances in the substrate are expected, i.e. $\lambda_{RA} = np_x$, and the solid black line corresponds to the resonance in the superstrate, i.e. $\lambda_{RAs} = np_{xs}$.

**Supporting-Information Figure S11**

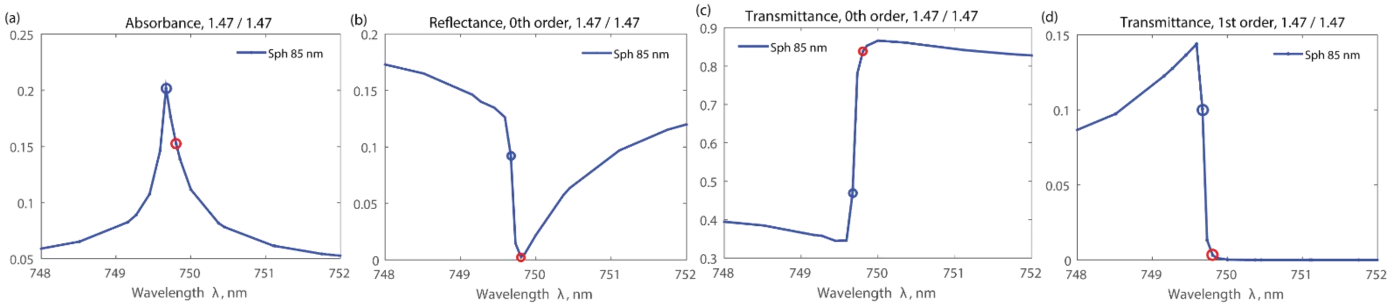


Fig. S11. (a) Absorbance of the nanoparticle array, (b) reflection in the zeroth order, transmission in (c) the zeroth and (d) the first orders of diffraction for sphere array with $R$ = 85 nm in the homogeneous environment with $n = n_s$ = 1.47 and narrow spectral range (wavelength 748-752 nm). Periods are $p_x$ = 510 nm and $p_y$ = 250 nm. Blue and red circles mark the maximum of absorbance and the minimum of reflectance, respectively. One can see that that reflectance minimum and transmittance maximum almost coincide with the maximum of absorbance, where EQ lattice resonance is excited.
